# Supplementary material for: Advanced creep modelling for polymers: A variable-order fractional calculus approach
Source: arXiv:2510.11765 source file (2025-10-13)
Supplement: Supplementary file 1 [file PaperPRSA2024_SM.pdf]

Supplementary Material for

# Advanced creep modeling for polymers: A variable-order fractional calculus approach

*José Geraldo Telles Ribeiro* [1] and Americo Cunha Jr [2,3]
[1]Rio de Janeiro State University, Department of Mechanical Engineering, Rio de Janeiro - RJ, 20550-900, Brazil
[2]Rio de Janeiro State University, Department of Applied Mathematics, Rio de Janeiro - RJ, 20550-900, Brazil
[2]National Laboratory of Scientific Computing, Petrópolis - RJ, 25651-075, Brazil

This document contains technical details about the model and results presented in the paper.

## 1. Phenomenological equation for the stress dependence of the model parameters

For every applied stress level $\sigma_0$ the six rheological quantities of the variable–order springpot model,

$$\{E,\, \eta,\, \beta_0,\, \beta_\infty,\, \gamma,\, \delta\},$$

are described through the empirical relation

$$P(\sigma_0) = \frac{(m_1\,\sigma_0 + m_2)\,(\sigma_0/\sigma_r)^n + m_3\,\sigma_0 + m_4}{(\sigma_0/\sigma_r)^n + 1}, \qquad P \in \{E, \eta, \beta_0, \beta_\infty, \gamma, \delta\}. \tag{S1}$$

Equation (S1) is a smoothed, four–coefficient rational-type interpolant able to reproduce monotonic, saturating or even weakly non-monotonic trends with only modest parameter correlation. Below we detail the physical meaning and dimensional consistency of the fitting constants for each $P$.

### Physical interpretation of the coefficients

The four parameters $m_1, m_2, m_3, m_4$ govern the asymptotic behavior and transition shape of the function $P(\sigma_0)$, as follows:

- **High-stress regime** ($\sigma_0 \gg \sigma_r$):

$$P(\sigma_0) \approx m_1\sigma_0 + m_2.$$

  - $m_1$: controls the *slope* of the high-stress asymptote.
  - $m_2$: defines the *intercept* of the high-stress asymptote.

- **Low-stress regime** ($\sigma_0 \ll \sigma_r$):

$$P(\sigma_0) \approx m_3\sigma_0 + m_4.$$

  - $m_3$: controls the *slope* of the low-stress asymptote.
  - $m_4$: defines the *intercept* of the low-stress asymptote.

- **Reference stress** $\sigma_r$: sets the stress level at which the transition between the low- and high-stress regimes occurs.
- **Exponent** $n$: tunes the sharpness of the transition between the two asymptotic regimes; larger $n$ results in a sharper transition.

Note: the coefficients $m_i$ have different physical units depending on the quantity being modeled.

## Elastic modulus $E(\sigma_0)$

- Unit of $E$: GPa
- $m_1$ and $m_3$ in MPa$^{-1}$
- $m_4$ and $m_2$ in GPa
- $n$ is dimensionless
- $\sigma_r$ in MPa

## Viscosity $\eta(\sigma_0)$

- Unit of $\eta$: GPa . s
- $m_1$ and $m_3$ in (MPa . s) $^{-1}$
- $m_4$ and $m_2$ in GPa . s
- $n$ is dimensionless
- $\sigma_r$ in MPa
- For the present study we imposed $\eta(\sigma_0) \equiv \eta_{\mathrm{ref}}$, so that $m_1 = m_2 = m_3 = 0$ and $m_4 = \eta_{\mathrm{ref}}$.

## Fractional orders $\beta_0(\sigma_0)$ and $\beta_\infty(\sigma_0)$

- Units of $\beta_0$ and $\beta_\infty$: dimensionless
- $m_1$ and $m_3$ in (MPa . s) $^{-1}$
- $m_4$ and $m_2$ are dimensionless
- $\sigma_r$ and $n$ as before

## Transition time $\gamma(\sigma_0)$

- Unit of $\gamma$: s
- $m_1$ and $m_3$ in (MPa . s) $^{-1}$
- $m_4$ and $m_2$ in s
- $\sigma_r$ and $n$ as before

## Shape exponent $\delta(\sigma_0)$

- Unit of $\delta$: dimensionless
- $m_1$ and $m_3$ in (MPa . s) $^{-1}$
- $m_4$ and $m_2$ are dimensionless
- $\sigma_r$ and $n$ as before

## Reference stress and curvature parameter

The pair $(\sigma_r, n)$ is *shared* by all six fits to guarantee a common inflection point and to mitigate over-parametrisation; $\sigma_r$ simply scales the stress axis, while $n$ dictates the sharpness of the transition between the two linear branches implicit in Eq. (S1).

Equation (S1) therefore offers a compact yet flexible description of the load dependence of every rheological parameter, ensuring dimensional correctness and minimal cross-correlation among the fitted coefficients.

## Fitting procedure and statistical confidence

All coefficients in (S1) were obtained by nonlinear least–squares minimization of the misfit function using the cross-entropy optimisation toolbox `CEopt` (Available at https://ceopt.org). Each parameter was bounded a priori within a physically admissible range (e.g. $0 < \beta_0, \beta_\infty < 1, E > 0$), and the search region was progressively tightened as the algorithm converged.

## Interpretation and practical use

Equation (S1) should be viewed as a stress-dependent *response surface* rather than as a fundamental constitutive rule. In numerical implementations one simply evaluates $P$ at the current value of $\sigma_0$ and feeds it to the time-domain governing equations (3.16)–(3.17).

Finally, we remark that the same functional form proved adequate for both polypropylene (PP) and polyvinyl-chloride (PVC) despite their markedly different magnitudes of $E$ and $\eta$. This suggests that (S1) may serve as a versatile template for other polymers or even metallic glasses, provided that the calibration data cover a sufficiently wide stress range.

## Remark on parameter inter–correlation.

Once the six stress–dependent surfaces $P(\sigma_0)$ have been identified through Eq.(S1), the simulation of the time–domain model (Eqs. (3.16)–(3.17)) becomes fully decoupled from the choice of the loading path. In other words, for any new stress level inside the calibrated envelope $2.8 < \sigma_0 < 12.6\,\mathrm{MPa}$ (PP) or $10 < \sigma_0 < 35\,\mathrm{MPa}$ (PVC) one simply queries Eq.(S1) to retrieve the appropriate $\{E, \eta, \beta_0, \beta_\infty, \gamma, \delta\}$ and solves the VO-Springpot equations without re-fitting. This feature is key to the *predictive* use of the model in design calculations.

## 2. Deformation curves for PP

Figure S1 juxtaposes the experimental creep curves (symbols) with the variable–order springpot predictions (solid lines. Both axes are shown in logarithmic scale to emphasise the three classical creep regimes. The model reproduces: (i) the nearly elastic plateau; (ii) the power-law drift in the transition zone; (iii) the steady-state slope, with a stress-dependent rate. All misfits remain below 1%, corroborating the load-independent viscosity hypothesis adopted in Section 4 of the main paper. The same curves in semilog-y scale are shown in Figure S2. A comparison between calibration and validation cases for PP, for different axis scales, is shown in Figure S3.

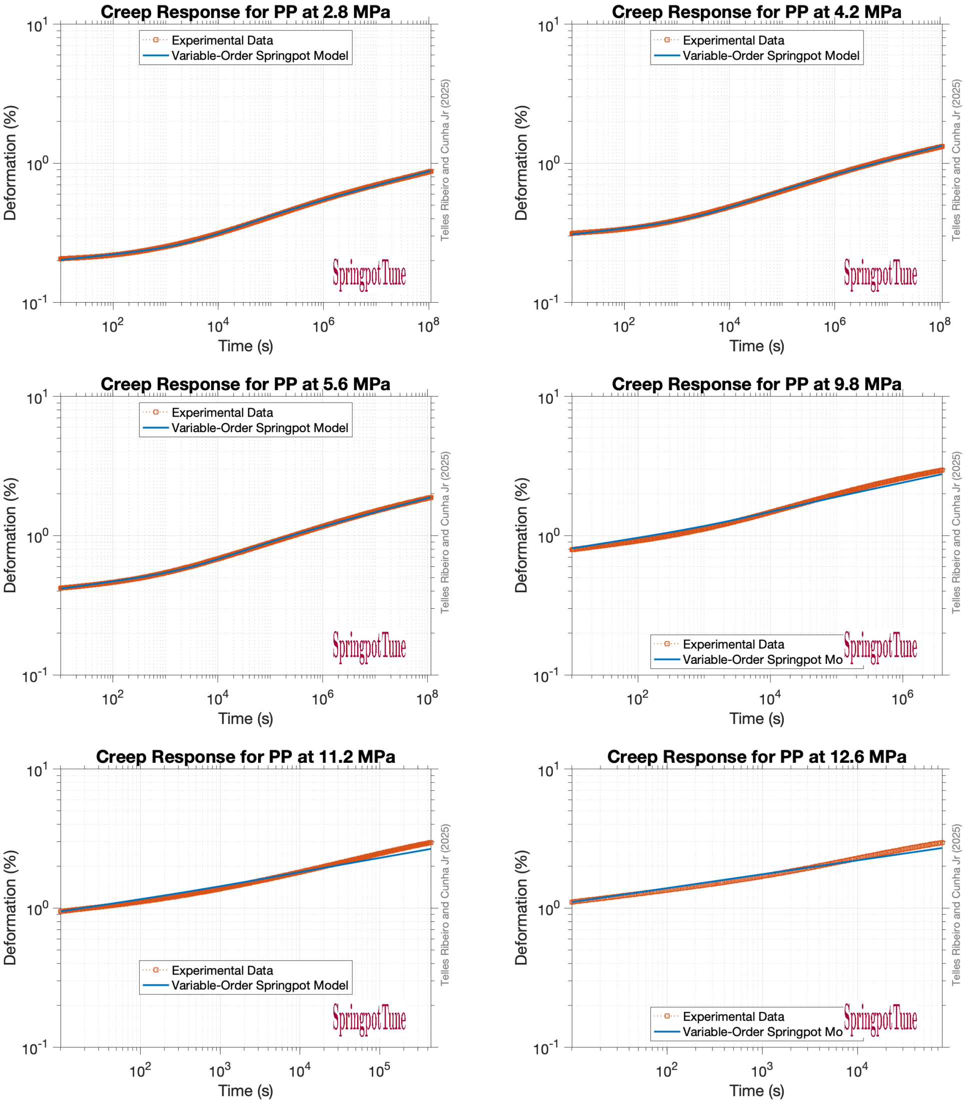


**Figure S1.** Predicted (*lines*) versus measured (*markers*) creep strain for PP at $20^{\circ}$C. Stress levels (MPa): 2.8, 4.2, 5.6, 9.8, 11.2, 12.6 (top to bottom). Log-log scale.

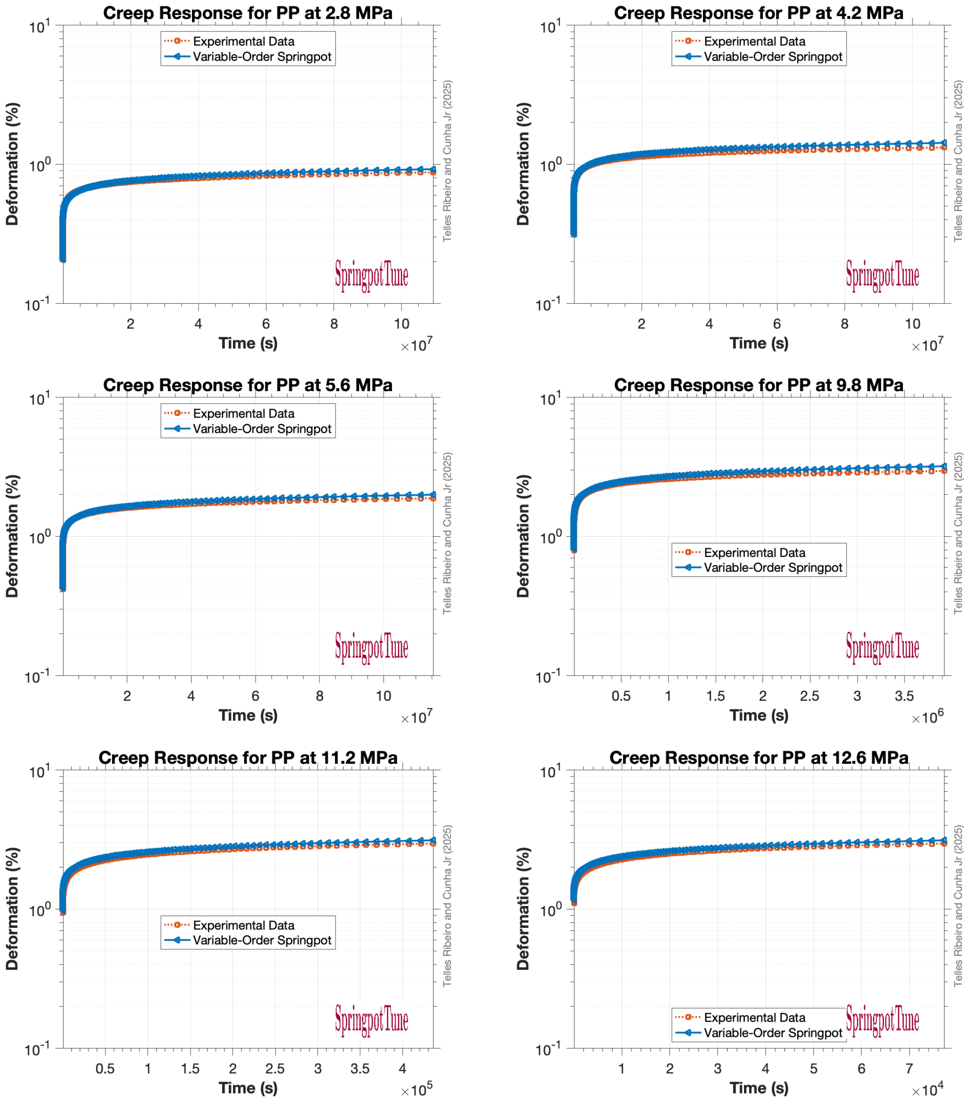


**Figure S2.** Predicted (*lines*) versus measured (*markers*) creep strain for PP at $20^{\circ}$C. Stress levels (MPa): 2.8, 4.2, 5.6, 9.8, 11.2, 12.6 (top to bottom). Semilog-y scale.

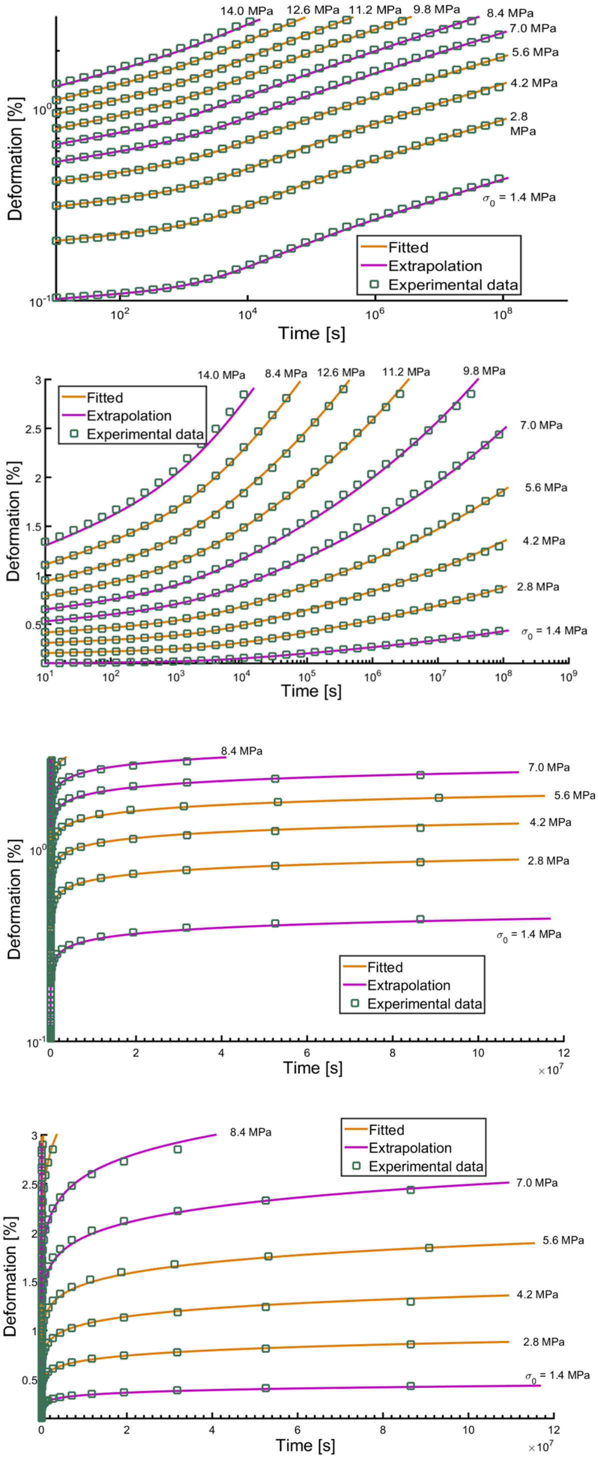


**Figure S3.** Creep curves of PP at 20 ℃ compared with the variable-order springpot model. From top to bottom: log-log scale; semilog-x scale; semilog-y scale; linear-linear scale. Solid lines are model predictions, symbols are experimental data.

## 3. Deformation curves for PVC

The same procedure was repeated for PVC; results are collected in Figure S4. Despite the two-order-of-magnitude increase in the reference viscosity ($\eta = 3 \times 10^5$ GPa s), the model captures the markedly faster transition from the glassy to the rubbery regime that is typical of PVC. Misfits stay below $1\%$ for the entire 10–35 MPa window, which further supports the robustness of Eq.(S1) as a *unified* stress surface for all six VO-Springpot parameters. The same curves in semilog-y scale are shown in Figure S5. same curves in semilog-y scale are shown in Figure S2. A comparison between calibration and validation cases for PVC, for different axis scales, is shown in Figure S6.

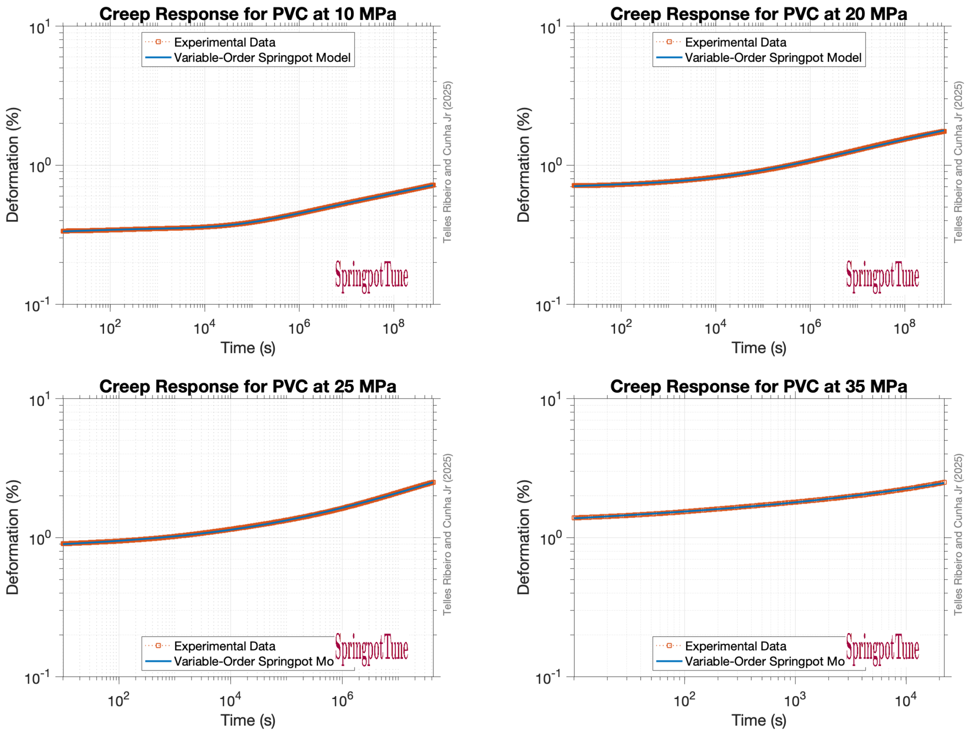


**Figure S4.** Predicted (*lines*) versus measured (*markers*) creep strain for PVC at $20^\circ$C. Stress levels (MPa): 10, 20, 25, 35 (top to bottom). Log-log scale.

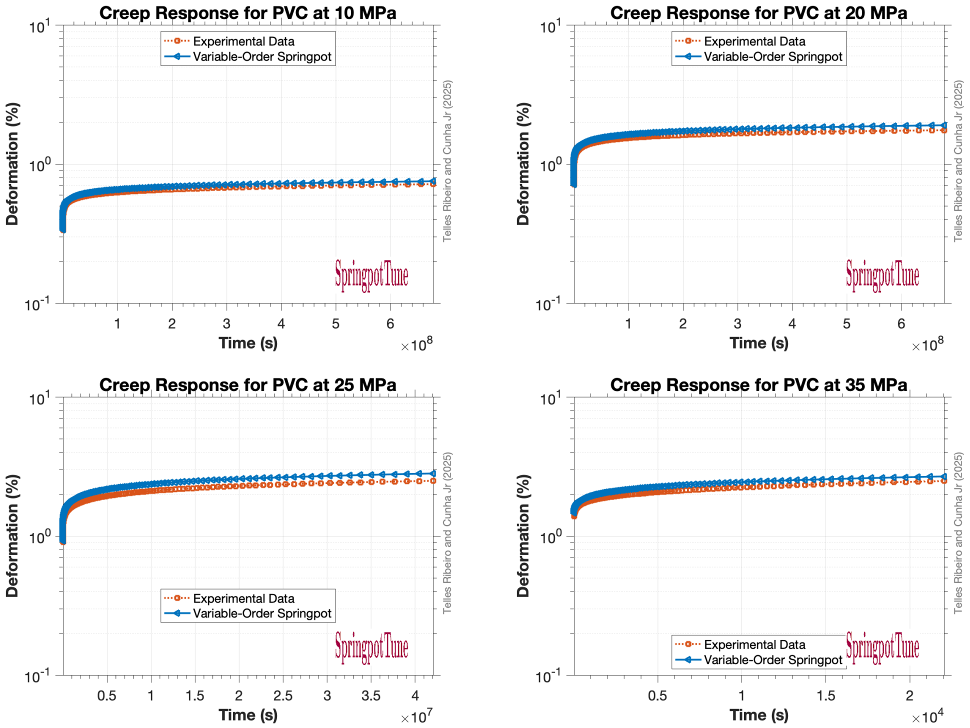


**Figure S5.** Predicted (*lines*) versus measured (*markers*) creep strain for PVC at $20^{\circ}$C. Stress levels (MPa): 10, 20, 25, 35 (top to bottom). Semilog-y scale.

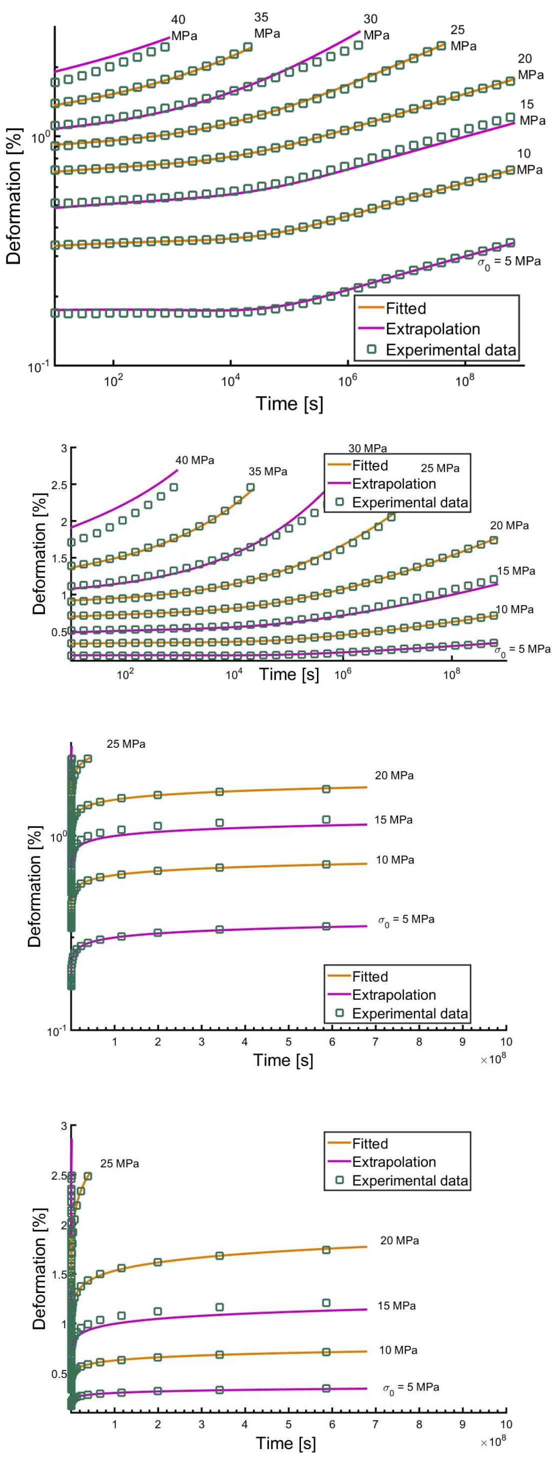


**Figure S6.** Creep curves of PVC at 20 ℃ compared with the variable-order springpot model. From top to bottom: log-log scale; semilog-x scale; semilog-y scale; linear-linear scale. Solid lines are model predictions, symbols are experimental data.

# 4. MATLAB® package SpringpotTune

All the programs used to calibrate and post-process the variable-order springpot model are openly available at an entirely self-contained GitHub repository:

https://americocunhajr.github.io/SpringpotTune

## The `CEopt.m` optimizer

`CEopt.m` is a self-contained MATLAB® routine that implements the cross–entropy (CE) algorithm for non-convex optimization. The purpose of the code is to solve

$$\min_{\mathbf{x}\in\mathbb{R}^{N_{\text{vars}}}} \; F(\mathbf{x}) \quad \text{s.t.} \quad \mathbf{lb} \le \mathbf{x} \le \mathbf{ub}, \qquad \mathbf{g}(\mathbf{x}) \le \mathbf{0}, \qquad \mathbf{h}(\mathbf{x}) = \mathbf{0},$$

where $F$ is a scalar objective function, and $\mathbf{g}$, $\mathbf{h}$ collect inequality and equality constraints.

**Call syntax** `[Xopt,Fopt,ExitFlag,CEstr] =`
`CEopt(fun,xmean0,sigma0,lb,ub,nonlcon,CEstr);`

**Inputs**
- `fun` – handle to the objective function ($1 \times N_{\text{vars}}$ row vector in, scalar out; may be vectorised);
- `xmean0, sigma0` – initial mean and std. dev. of the sampling Gaussian;
- `lb, ub` – lower/upper bounds;
- `nonlcon` – optional handle returning $[\mathbf{g}(\mathbf{x}), \mathbf{h}(\mathbf{x})]$;
- `CEstr` – structure with CE settings (see below).

**Important `CEstr` fields**

| | |
|---|---|
| `Nvars` | number of decision variables; |
| `EliteFactor` | elite fraction $\rho$ ($\approx 0.05$); |
| `Nsamp` | samples per generation; |
| `MaxIter` | maximum CE iterations; |
| `MaxFcount` | budget of calls to `fun`; |
| `TolAbs,TolRel` | absolute/relative tolerance on $F$; |
| `alpha,beta` | smoothing factors for mean / std. dev.; |
| `isConstrained` | indicate if the problem is constrained. |

**Outputs**
- `Xopt` – best point found;
- `Fopt` – corresponding objective value;
- `ExitFlag` – reason for termination;
- `CEstr` – the updated structure containing complete trajectories of $\boldsymbol{\mu}_k$, $\boldsymbol{\sigma}_k$, $\mathbf{x}_{\text{best}}$, objective statistics, constraint errors, etc.

**Algorithmic steps**
- (i) **Initialisation** with Gaussian $\mathcal{N}(\boldsymbol{\mu}_0, \boldsymbol{\sigma}_0^2)$ truncated to $(\mathbf{lb}, \mathbf{ub})$;
- (ii) **Sampling** – draw `Nsamp` points;
- (iii) **Feasibility check** – projects/penalises points that violate bounds or nonlinear constraints;
- (iv) **Elite selection** – keep the $\rho$ % best samples;
- (v) **Parameter update**

$$\boldsymbol{\mu}_{k+1} = (1-\alpha)\,\boldsymbol{\mu}_k + \alpha\,\hat{\boldsymbol{\mu}}, \qquad \boldsymbol{\sigma}_{k+1} = (1-\beta)\,\boldsymbol{\sigma}_k + \beta\,\hat{\boldsymbol{\sigma}},$$

  where $\hat{\cdot}$ denotes elite statistics;
- (vi) **Stopping checks** against tolerances, stall counters, function value targets, or maximum resources.

**License** GNU GPL v3; see header of the file for details.

## The `Main_VOSpringpot_Calibration1.m` script

- *Input*
  - creep data at many loads, stored in `CreepDataPP.csv` or `CreepDataPVC.csv` (columns: load, time [day], strain [%]);
  - user–selected load $\sigma_0$;
  - loose lower/upper bounds for the six VO–springpot parameters $\{E, \eta, \beta_0, \beta_\infty, \gamma, \delta\}$.
- *Process*
  (i) extracts the $(t, \varepsilon_{\text{exp}})$ subset corresponding to $\sigma_0$ and converts time to seconds;
  (ii) defines the misfit function $J(\mathbf{x}) =$;
  (iii) minimises $J$ with `CEopt`;
  (iv) writes `VOSpringpotParameters_*.csv` and the calibrated creep curve figure.
- *Output plot* — `PlotLoglog2`: experimental strain (`:`) vs. calibrated model (–) in a log–log diagram.

## The `Main_VOSpringpot_Calibration2.m` script

- Starts from the point–wise parameters obtained with `Calibration1`.
- For a user-selected material parameter (e. g. $E$ or $\gamma$) it minimises the residuals between the discrete values and the phenomenological law (Eq. (4.1) in the main text);
- Uses the same CE machinery (bounds now refer to $\{\sigma_r, n, m_1, \ldots, m_4\}$);
- Generates a `Plot2` figure: symbols for fitted points, solid line for the phenomenological curve (linear–linear or semi-log scale depending on the parameter).

## The `Main_VOSpringpot_StrainCurves.m` script

- Reads the raw creep database and prompts the user for a load $\sigma_0$;
- Evaluates *all* VO–springpot parameters at that $\sigma_0$ by calling the calibrated phenomenological laws (output of `Calibration2`);
- Simulates the strain history with the analytical formula

$$\varepsilon(t) = \frac{\sigma_0}{E\,\Gamma[\beta(t)+1]}\,[t/T]^{\beta(t)}, \qquad \beta(t) = \frac{\beta_\infty (t/\gamma)^\delta + \beta_0}{(t/\gamma)^\delta + 1},$$

  where $T = \eta/E$;
- Plots experimental data and prediction in either `log-log` or `semi-logy` mode (routine `PlotLoglog2` or `PlotSemilogy2`).

## Utility functions

**`DeformationEq(x,t)`** returns the analytical strain for a parameter vector `x` and time grid `t`;
**`PhenomEq(`**$\sigma_0, \sigma_r, n, m_1 \ldots m_4$**`)`** implements Eq. (4.1) for a single load value;
**`Plot{Loglog2,Semilogx2,Semilogy2}`** uniform wrappers that enforce the colour palette, legend, signature line and file export.

> Every script is fully vectorised, reproduces the figures with one click, and was tested under MATLAB R2022b on Windows, macOS and Linux.
